# Supplementary material for: End-to-end View Synthesis via NeRF Attention
Source: arXiv:2207.14741 source file (2022-09-15)
Supplement: Supplementary file 1 [file appendix.tex]

\section{More Visualizations}
We visualize the results on the CO3D~\cite{nerformer} dataset in Figure~\ref{Fig:co3d_plant} and Figure~\ref{Fig:co3d_suitcase}. A video comparing NeRF and NeRFA is provided in the supplementary.
\begin{figure}[!t]
  \centering
  \includegraphics[width=\textwidth]{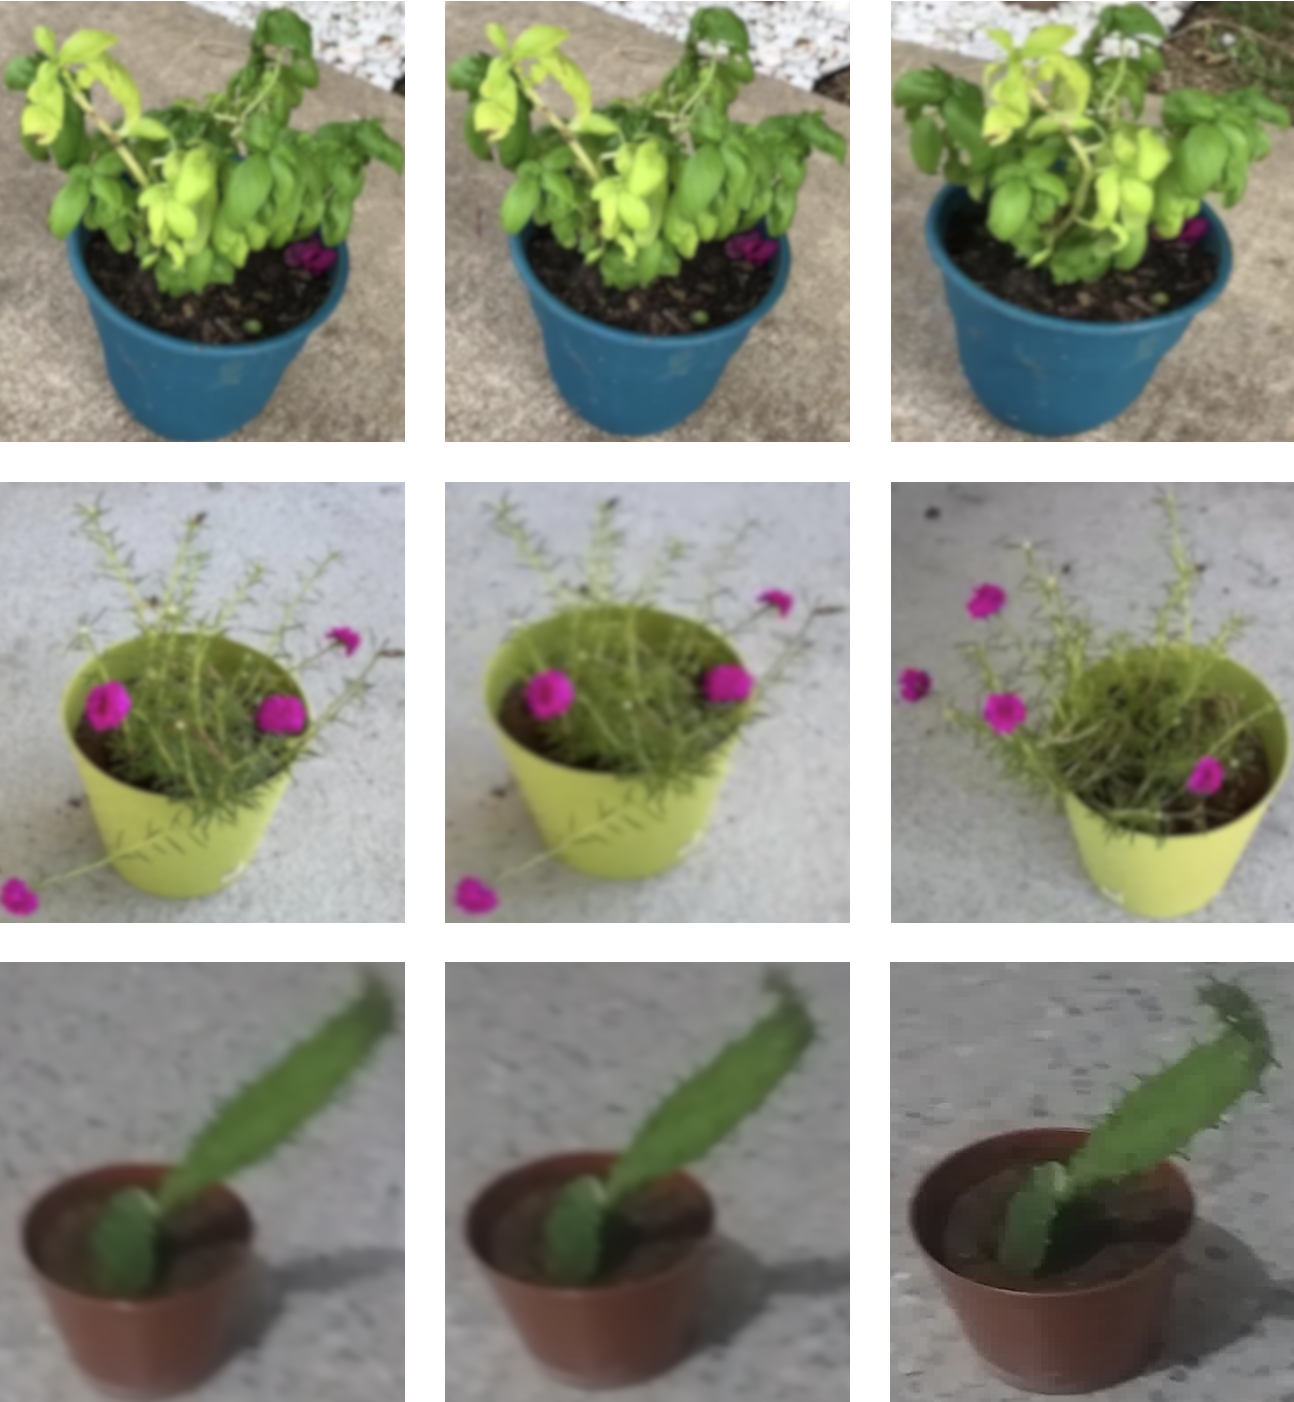}
  \caption{Category-centric view synthesis results of the plant category on the CO3D~\cite{nerformer} dataset. Each row corresponds to a view. The first row is from the $\texttt{train-unseen}$ split and the other rows are from the $\texttt{test-unseen}$ split.}
  \label{Fig:co3d_plant}
\end{figure}

\begin{figure}[!t]
  \centering
  \includegraphics[width=\textwidth]{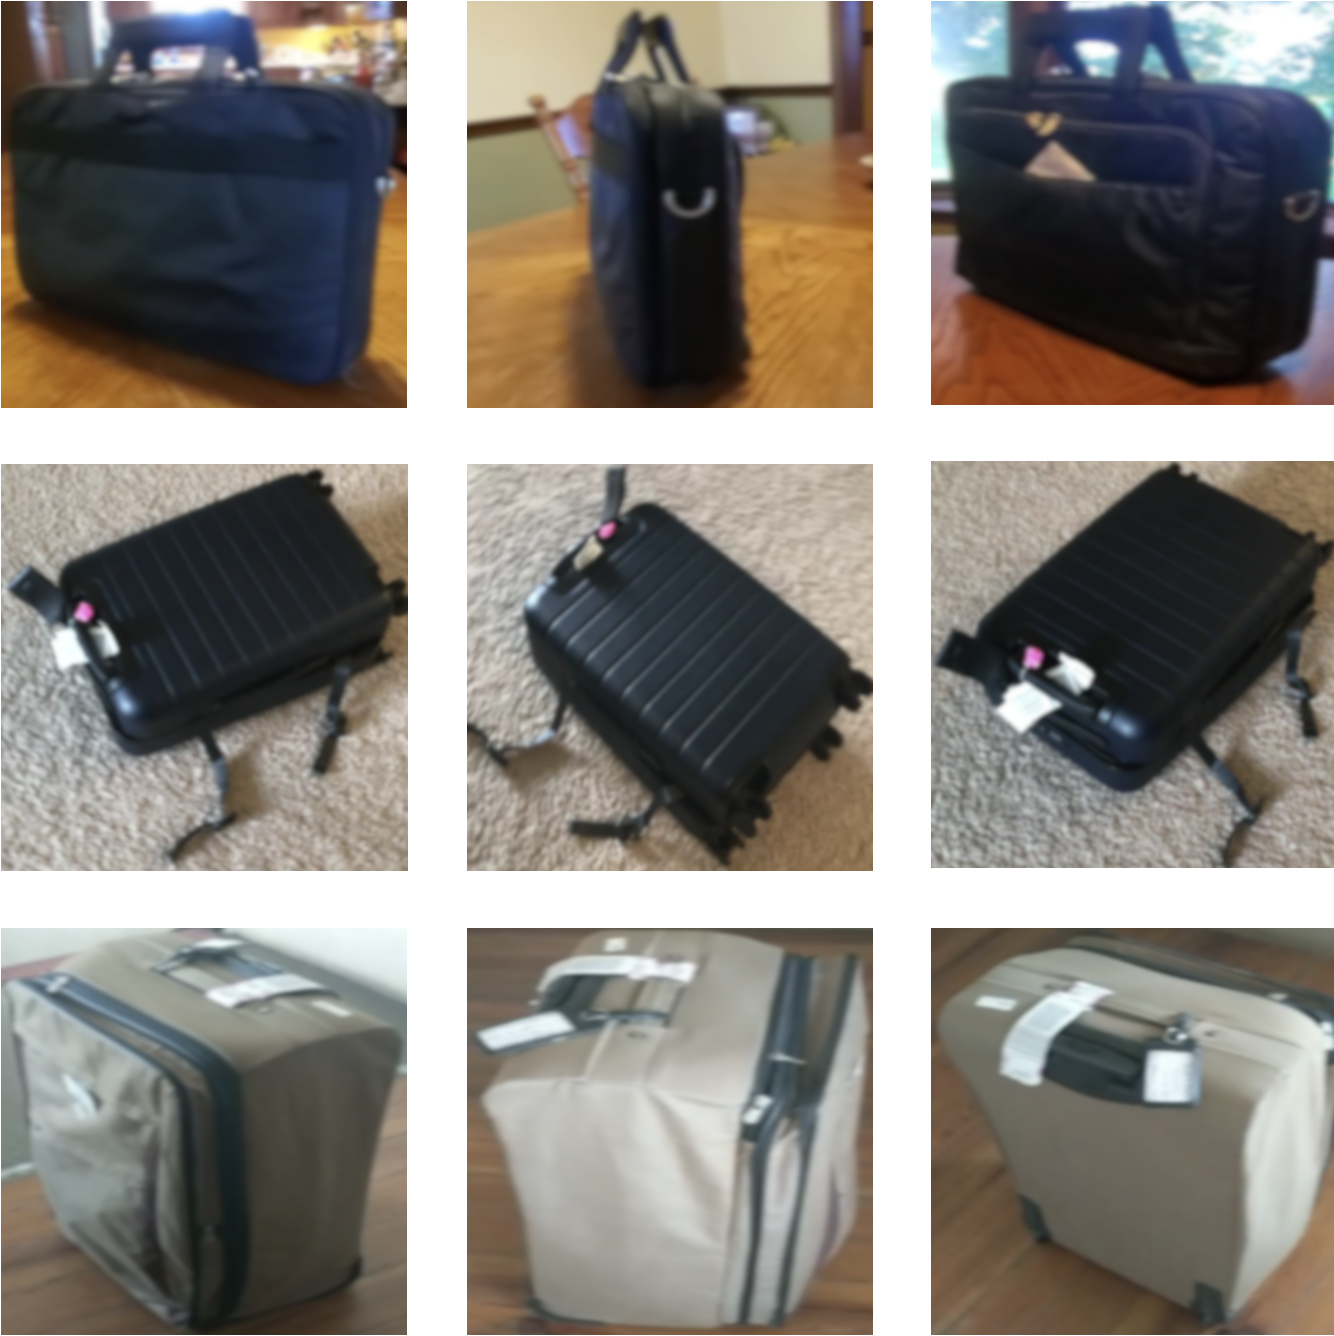}
  \caption{Category-centric view synthesis results of the suitcase category on the CO3D~\cite{nerformer} dataset. Each row corresponds to a view. The first row is from the $\texttt{train-unseen}$ split and the other rows are from the $\texttt{test-unseen}$ split.}
  \label{Fig:co3d_suitcase}
\end{figure}

\section{Computational Resources}
We train our model and the baselines on a 48-core Ubuntu 16.04 Linux server with one Nvidia V100 GPU. The CPU is Intel Silver 4116 CPU @ 2.10GHz. The training time for one model is approximately three days.

\section{License and Permissions}
The DeepVoxels~\cite{deepvoxels_sitzmann}, Blender~\cite{nerf} and LLFF~\cite{localLightFieldFusion} dataset are built upon the Creative Commons Attribution (CC-BY) licence. The CO3D dataset~\cite{nerformer} is built upon the BSD license. No offensive components are found in these datasets. The creators are properly cited in the main text.

\section{Limitations}
\label{ap:limitations}
Despite our contributions to seq2seq formulation and NeRFA models, our work has several limitations. First, the NeRFA model needs more training time than NeRF. However, we believe that foundation models such as transformers~\cite{foundationModels} are worth exploring because of their strong generalization ability. Second, we hypothesize that one can still improve NeRFA's architecture design since the community has not exploited the power of transformers. We would incorporate recent advances in transformers \cite{SwinTransformer, largeBert} to improve NeRFA. Furthermore, we could conduct deeper ablation studies to understand the importance of different components in NeRFA. 

\section{Broader Impact}
\label{ap:negBroader}
Our findings provide a simple yet effective approach to addressing view synthesis problems. Potentially, people may leverage the NeRFA models to generate novel views. However, the learned transformers may be attacked by adversarial training \cite{AdversarialAttacks}. And attackers may use the synthesized views to deceive people because the synthesized views are too realistic. However, these potential negative impacts are not restricted to our work but also appear in prior works~\cite{nerf,mip_nerf} as well. Practitioners must take care of the view synthesis approaches to avoid possible negative influences.
